# Supplementary material for: Lying Your Way to Better Traffic Engineering
Source: arXiv:1610.02728 source file (2016-11-01)
Supplement: Supplementary file 1 [file 700-appendix-golden-ratio.tex]

\section{Compunting the Optimal Oblivious Routing of the Motivating Example}\label{sect:app-golden-ratio}

We show how to compute the optimal per-destination routing for the example instance of Fig.~\ref{fig:COYOTE-overview}. 
We first observe that the set of demands for which the routing must be optimised can be reduced to the vertices of the 
polyhedral representing those demands that can be routed with congestion at most 1. Namely, we consider two demands
$d_1=\{(s_1,s_2)=(2,0)\}$ and $d_1=\{(s_1,s_2)=(0,2)\}$.
We denote by $load(e)$ the amount of flow routed on edge $e$. 
We observe that $load(s_1,v)\le load(v,t)$ and $load(s_2,v)\le load(v,t)$ since link $(v,t)$ routes the same flow through $(s_1,v)$ plus the flow
from $(s_2,v)$.

Hence, given $d_1$, we the most congested edge is must be either $(s_1,s_2)$ or $(v,t)$: 

$$load(s_1,s_2)\ge 2 \Phi(s_1,s_2)$$
$$load(v,t)\ge 2(1 - \Phi(s_1,s_2)) + 2\Phi(s_1,s_2) (1-\Phi(s_2,t)) = 2(1 - \Phi(s_1,s_2) \Phi(s_2,t))$$

As for demand $d_2$, we observe that the most congested edge is either $(s_2,t)$ or $(v,t)$, where:

$$load(s_2,t)\ge 2 \Phi(s_2,t)$$
$$load(v,t)\ge 2(1 - \Phi(s_2,t))$$

As for $load(v,t)$, we observe that $ 2(1 - \Phi(s_1,s_2) \Phi(s_2,t)) \ge  2(1 - \Phi(s_2,t))$, for any $0\le \Phi(s_2,t) \le 1$, which
means that $load(v,t)\ge 2(1 - \Phi(s_2,t))$ is obsolete.

We want to balance the congestion among these two demands on $(s_1,s_2)$, $(s_2,t)$, and $(v,t)$. 

By a case-by-case analysis, it is easy to observe that all the following three inequalities must be tight in the optimal case:

$$load(s_1,s_2)\ge 2 \Phi(s_1,s_2)$$
$$load(v,t)\ge 2(1 - \Phi(s_1,s_2) \Phi(s_2,t))$$
$$load(v,t)\ge 2\Phi(s_2,t)$$

Hence, we have that the $load(v,t)$ equations leads to:

$$2\Phi(s_2,t)= 2(1 - \Phi(s_1,s_2) \Phi(s_2,t))$$

Since $load(s_1,s_2)=load(v,t)$, we have that $ \Phi(s_1,s_2)= \Phi(s_2,t)$, which leads to:

$$\Phi(s_1,s_2)= 1 - \Phi(s_1,s_2)^2$$

$$1 - \Phi(s_1,s_2) -\Phi(s_1,s_2)^2=0$$

\noindent
, which is an equation of the second order with solutions:

$$\Phi(s_1,s_2)=\frac{\sqrt{5}-1}{2} \sim 1,618 \mbox{ and } \Phi(s_1,s_2)=\frac{\sqrt{5}+1}{2} \sim 0,618$$

\noindent
, where only the second solution (i.e., the inverse of the golden ratio) is feasible in our formulation. The optimal splitting ratios are therefore:

$$ \Phi(s_1,s_2)= \frac{\sqrt{5}-1}{2} \mbox{ and } \Phi(s_2,t)= -\frac{\sqrt{5}+1}{2}  $$

\noindent
where the most congested edge for any permitted traffic matrix is at most $\sqrt{5}-1\sim 1,23$. COYOTE correctly finds this solution.
